# Supplementary material for: Competing orders and cascade of degeneracy lifting in doped Bernal bilayer graphene
Source: arXiv:2111.15673 ancillary file (2022-05-06)
Supplement: Supplementary file 1 [file BLG_Supplementary.pdf]

# Supplementary Material: Competing orders and cascade of degeneracy lifting in doped Bernal bilayer graphene

András L. Szabó[1] and Bitan Roy[2]

[1] Max-Planck-Institut für Physik komplexer Systeme, Nöthnitzer Str. 38, 01187 Dresden, Germany

[2] Department of Physics, Lehigh University, Bethlehem, Pennsylvania, 18015, USA

(Dated: November 30, 2021)

The Supplementary Material contains: (1) Definition of Nambu-doubled spinor. (2) Computation of renormalization group flow equations. (3) Pairing matrices in the presence of in-plane magnetic field, appearing in their susceptibility calculation.

## S1. NAMBU-DOUBLED SPINOR

The sixteen-component Nambu-doubled spinor in Bernal bilayer graphene is defined as

$$\Psi_{\rm Nam} = \begin{pmatrix} \Psi_{\omega,\boldsymbol{k}} \\ \Gamma_{210}\Psi^*_{-\omega,-\boldsymbol{k}} \end{pmatrix}, \tag{S1}$$

where in the lower block we absorbed the unitary part of the time reversal operator $U = \Gamma_{210} \equiv \sigma_2\tau_1\beta_0$. The eight-component spinor is

$$\Psi_{\omega,\boldsymbol{k}} = \left[c_\uparrow^{+K}, c_\uparrow^{-K}, c_\downarrow^{+K}, c_\downarrow^{-K}\right]^\top(\omega), \text{ with } c_s^v = \left[a_{2,s}^v, b_{1,s}^v\right]. \tag{S2}$$

Here $r^v_{j,s}(\omega)$ are annihilation operators for fermions on the $a_2$ and $b_1$ sublattices with valley index $v = \pm\boldsymbol{K}$, Matsubara frequency $\omega$, spin projection $s = \uparrow, \downarrow$, and $\top$ denotes transposition. In the main manuscript $\Psi \equiv \Psi_{\rm Nam}$.

## S2. RENORMALIZATION GROUP ANALYSIS

The Green's function for quadratic fermions subject to Zeeman field $h$ in the announced Nambu basis is

$$G(i\omega_n,\boldsymbol{k}) = \text{diag.}\Bigg[\frac{i\omega_n-\mu+h-d_1\Gamma_{01}-d_2\Gamma_{32}-u\Gamma_{03}}{(i\omega_n-\mu+h)^2-E_u^2}, \frac{i\omega_n-\mu-h-d_1\Gamma_{01}-d_2\Gamma_{32}-u\Gamma_{03}}{(i\omega_n-\mu-h)^2-E_u^2},$$
$$\frac{i\omega_n+\mu+h+d_1\Gamma_{01}+d_2\Gamma_{32}+u\Gamma_{03}}{(i\omega_n+\mu+h)^2-E_u^2}, \frac{i\omega_n+\mu-h+d_1\Gamma_{01}+d_2\Gamma_{32}+u\Gamma_{03}}{(i\omega_n+\mu-h)^2-E_u^2}\Bigg], \tag{S3}$$

where $E_u = \sqrt{k^4/(4m_*^2)+u^2}$, $\Gamma_{\nu\rho} = \tau_\nu\beta_\rho$, and $d_i \equiv d_i(\boldsymbol{k})$ $(i = 1,2)$ are $d$-wave harmonics defined in the main text.

Let us start with the renormalization of the interaction coupling in the $E_g$ channel. The interacting Lagrangian is

$$L_{\rm int} = g_{_{E_g}} \sum_{i=1}^{2} (\Psi^\dagger M_i \Psi)^2, \tag{S4}$$

where $M_1 = \Gamma_{3001}$ and $M_2 = \Gamma_{3032}$. The contributions of the four one-loop diagrams [see Fig. S1(a)], namely bubble $(B)$, vertex $(V)$, crossing $(C)$, and ladder $(L)$ are respectively

$$B = 2t \sum_{n=-\infty}^{\infty} \int_{\Lambda e^{-\ell}}^{\Lambda} \frac{{\rm d}k\; k}{(2\pi)^2} \int_0^{2\pi} {\rm d}\phi {\rm Tr}\Big[-\sum_{i=1}^{2} M_i G(i\omega_n,\boldsymbol{k}) M_i G(i\omega_n,\boldsymbol{k})\Big],$$

$$V = 4t \sum_{n=-\infty}^{\infty} \int_{\Lambda e^{-\ell}}^{\Lambda} \frac{{\rm d}k\; k}{(2\pi)^2} \int_0^{2\pi} {\rm d}\phi \frac{1}{16} {\rm Tr}\Big[M_k \sum_{i=1}^{2} M_i G(i\omega_n,\boldsymbol{k}) M_k G(i\omega_n,\boldsymbol{k}) M_i\Big],$$

$$C = 2t \sum_{n=-\infty}^{\infty} \int_{\Lambda e^{-\ell}}^{\Lambda} \frac{{\rm d}k\; k}{(2\pi)^2} \int_0^{2\pi} {\rm d}\phi \sum_{i,j=1}^{2} \frac{1}{(16)^2} {\rm Tr}\Big[M_k M_i G(i\omega_n,\boldsymbol{k}) M_j\Big] {\rm Tr}\Big[M_k M_j G(i\omega_n,\boldsymbol{k}) M_i\Big],$$

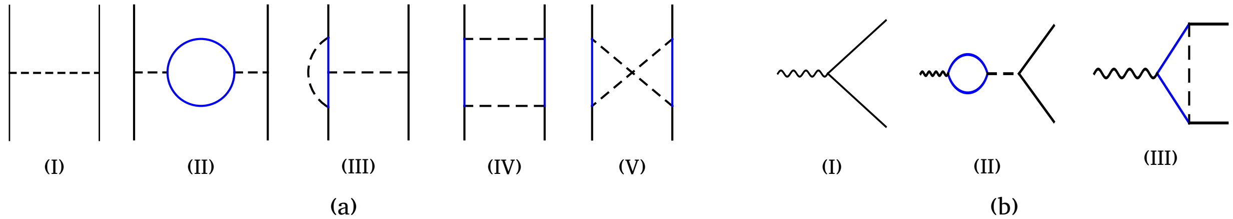


Figure S1. (a) Feynman diagrams yielding renormalization of quartic coupling. (aI) Bare four-fermion interaction vertex. Feynman diagrams (aII)-(aV) yield corrections to the bare interaction vertex to the leading order. Here, solid lines represent fermions. While the blue lines in (aII)-(aV) correspond to the fast modes, living within a thin Wilsonian momentum shell $\Lambda\ e^{-\ell} < |\mathbf{k}| < \Lambda$, where $\Lambda$ is the ultraviolet momentum cut-off and $\ell$ is the logarithm of the renormalization group scale, the black solid lines are the slow modes with $|\mathbf{k}| < \Lambda\ e^{-\ell}$. (b) Feynman diagrams yielding renormalization of conjugate field. (bI) The bare source term vertex. The leading order renormalization of such vertex arises from Feynman diagrams (bII) and (bIII), yielding the RG flow of the source terms or conjugate fields. Here, wavy lines stand for the conjugate field, while solid lines for fermions, and the dashed lines for the interaction vertex.

$$L = 2t \sum_{n=-\infty}^{\infty} \int_{\Lambda e^{-\ell}}^{\Lambda} \frac{\mathrm{d}k\ k}{(2\pi)^2} \int_0^{2\pi} \mathrm{d}\phi \sum_{i,j=1}^{2} \frac{1}{(16)^2} \mathrm{Tr}\Big[M_k M_i G(i\omega_n, \boldsymbol{k}) M_j\Big] \mathrm{Tr}\Big[M_k M_i G(-i\omega_n, -\boldsymbol{k}) M_j\Big], \tag{S5}$$

where $k = 1$ or 2. The evaluation of the above contributions is as follows.

1. First we compute the angular integral over $\phi$, which yields $\pi$ for terms proportional to $d_i^2$ $(i = 1, 2)$. All other nonvanishing terms are independent of $\phi$ and we then obtain a factor of $2\pi$.

2. Next we perform the summations over the Matsubara frequencies $\omega_n = (2n + 1)\pi t$, that have closed analytical forms. These are however lengthy and not particularly instructive. Therefore, we do not show their explicit forms.

3. The remaining integral runs across the thin momentum shell $\Lambda e^{-\ell} < |\boldsymbol{k}| < \Lambda$, where $\ell \ll 1$. We perform it as

$$\int_{\Lambda e^{-\ell}}^{\Lambda} \mathrm{d}k f(k) \approx f(\Lambda)\Lambda\ell. \tag{S6}$$

4. Finally, we define dimensionless variables as

$$\frac{2m_* g_{E_g}}{8\pi} \to \lambda_{E_g}, \qquad \frac{2m_* x}{\Lambda^2} \to \tilde{x}, \tag{S7}$$

where $x = t, \mu, u, h$. The RG flow equation of the coupling constant $\lambda_{E_g}$ then reads

$$\frac{\mathrm{d}\lambda_{E_g}}{\mathrm{d}\ell} = \lambda_{E_g}^2 (B + V + C + L) \equiv \lambda_{E_g}^2 H(t, \mu, u, h), \tag{S8}$$

after taking $\tilde{x} \to x$ for notational simplicity, as defined in Eq. (5) of the main text.

Next we show the renormalization of conjugate fields $\Delta_y$ coupling to a fermion bilinear as $\Delta_y(\Psi^\dagger N_y \Psi)$ for $y = E_g$, $A_{1g}$, $A_{1u}^{\parallel}$, $A_{1u}^{\perp}$. The explicit form of the bilinear order parameters is

$$\Delta_{E_g}\left[\Psi^\dagger \Gamma_{3001}\Psi + \Psi^\dagger \Gamma_{3032}\Psi\right], \quad \Delta_{A_{1g}} \sum_{\mu=1,2} \Psi^\dagger \Gamma_{\mu 000}\Psi, \quad \Delta_{A_{1u}^{\parallel}} \sum_{\mu=1,2} \Psi^\dagger \Gamma_{\mu 330}\Psi, \ \text{ and } \ \Delta_{A_{1u}^{\perp}} \sum_{\mu=1,2}\sum_{j=1,2} \Psi^\dagger \Gamma_{\mu j 30}\Psi.$$

Here $\Delta_{A_{1u}^{\parallel}}$ ($\Delta_{A_{1u}^{\perp}}$) couples with the component of the $f$-wave pairing parallel (perpendicular) to the direction of the external in-plane magnetic fields. Two one-loop diagram [Fig. S1(b)] contributions bubble ($B_y$) and vertex ($V_y$) read

$$\begin{aligned} B_y &= 2t \sum_{n=-\infty}^{\infty} \int_{\Lambda e^{-\ell}}^{\Lambda} \frac{\mathrm{d}k\ k}{(2\pi)^2} \int_0^{2\pi} \mathrm{d}\phi \mathrm{Tr}\Big[-\sum_{i=1}^{2} M_i G(i\omega_n, \boldsymbol{k}) N_y G(i\omega_n, \boldsymbol{k})\Big], \\ V_y &= 2t \sum_{n=-\infty}^{\infty} \int_{\Lambda e^{-\ell}}^{\Lambda} \frac{\mathrm{d}k\ k}{(2\pi)^2} \int_0^{2\pi} \mathrm{d}\phi \frac{1}{16} \mathrm{Tr}\Big[N_y \sum_{i=1}^{2} M_i G(i\omega_n, \boldsymbol{k}) N_y G(i\omega_n, \boldsymbol{k}) M_i\Big], \end{aligned} \tag{S9}$$

respectively. The evaluation of the above loop integrals is analogous to those renormalizing the interaction coupling. The $\beta$-functions of conjugate fields then become

$$\frac{\mathrm{d}\ln \Delta_y}{\mathrm{d}\ell} - 2 = \lambda_{E_g}(B_y + V_y) \equiv \lambda_{E_g} J_y(t, \mu, u, h), \tag{S10}$$

as defined in Eq. (6) of the main text.

## S3. SUSCEPTIBILITY CALCULATION

Next we present details of the susceptibility calculation. Recall that the bare mean-field susceptibility for zero external momenta and frequency reads

$$\chi = -t \sum_{n=-\infty}^{\infty} \int \frac{d^2\boldsymbol{k}}{(2\pi)^2} \mathrm{Tr}\left[G(i\omega_n, \boldsymbol{k}) M G(i\omega_n, \boldsymbol{k}) M\right]. \tag{S11}$$

The $M$ matrices transforming under various irreducible representations of the $D_{3d}$ group are shown below, where we collect spin singlet and spin triplet pairing matrices separately.

$$\text{singlet} = \begin{cases} A_{1g}: & M = \Gamma_{\mu 000} \\ E_g: & M = \{\Gamma_{\mu 001}, \Gamma_{\mu 032}\} \\ A_{2u}: & M = \Gamma_{\mu 003} \\ A_{1\mathbf{K}}: & M = \{\Gamma_{\mu 011}, \Gamma_{\mu 021}\} \\ E_{\mathbf{K}}: & M = \{\Gamma_{\mu 010}, \Gamma_{\mu 013}, \Gamma_{\mu 020}, \Gamma_{\mu 023}\} \end{cases}$$

$$\text{triplet} = \begin{cases} A_{2g}: & M = \{\Gamma_{\mu 133}, \Gamma_{\mu 233}, \Gamma_{\mu 333}\} \\ A_{1u}: & M = \{\Gamma_{\mu 130}, \Gamma_{\mu 230}, \Gamma_{\mu 330}\} \\ E_u: & M = \{\Gamma_{\mu 131}, \Gamma_{\mu 102}, \Gamma_{\mu 231}, \Gamma_{\mu 202}, \Gamma_{\mu 331}, \Gamma_{\mu 302}\} \\ A_{2\mathbf{K}}: & M = \{\Gamma_{\mu 112}, \Gamma_{\mu 122}, \Gamma_{\mu 212}, \Gamma_{\mu 222}, \Gamma_{\mu 312}, \Gamma_{\mu 322}\} \end{cases}$$

Here $\mu = 1, 2$ reflects the superconducting U(1) gauge degree of freedom. Without the loss of generality, for the calculation of the susceptibility we set $\mu = 1$. Among spin triplet pairing matrices, the spin component parallel to the layer antiferromagnet (ferromagnet) ordering is shown in blue (black). The spin component perpendicular to both layer antiferromagnet and ferromagnet ordering is shown in red.
